# Supplementary material for: Anomalous Behavior in the Nucleation of Ice at Negative Pressures
Source: arXiv:2401.12896 source file (2024-01-23)
Supplement: Supplementary file 1 [file SM_final.pdf]

# Supporting Material of: Anomalous behavior in the nucleation of ice at negative pressures

Valentino Bianco<sup>1</sup>, Pablo Montero de Hijes<sup>1</sup>, Cintia P. Lamas<sup>1</sup>, Eduardo Sanz<sup>1</sup>, Carlos Vega<sup>1</sup>  
<sup>1</sup> *Faculty of Chemistry, Chemical Physics Department, Universidad Complutense de Madrid,  
Plaza de las Ciencias, Ciudad Universitaria, Madrid 28040, Spain\**

---

\* vabianco@ucm.es, cvega@ucm.es

## DIRECT COEXISTENCE SIMULATIONS

To determine the solid-liquid equilibrium line we place a block of ice Ih consisting of 4032 molecules in contact with an equal number of liquid molecules. We perform  $NPT$  simulations, with anisotropic  $P$  to relax the crystal structure, counting the number of solid molecules in time. Along an isobar, if  $T$  is larger than the coexistence temperature the ice melts, hence the number of solid particles decreases in time. On the other hand, for  $T$  below the coexistence temperature the number of solid molecules increases in time. The coexistence  $T$  is determined when, for independent trajectories, the ice shows equal probability of melting or growing.

## SEEDING SIMULATIONS

The purpose of this technique is to find the critical nucleus size at a certain temperature  $T$  and pressure  $P$ . Given that the critical nucleus is situated at the top of the energy barrier, it is in unstable equilibrium and the probability for the nucleus to grow or to shrink is equally 50%. Therefore, by inserting a crystal seed of a given size  $N$  within the bulk liquid and tracking its evolution with time over multiple independent runs, we can estimate if  $N$  is larger than the critical size  $N_c$  (meaning that all the crystal seeds grow) or if it is smaller (in which case all the seeds melt). When  $N \sim N_c$  we expect to observe the ice growing for half of the trajectories, and melting for the remaining ones.

Introduced in 2005 [1], the *seeding* technique's popularity has grown over the last few years being extensively applied in nucleation studies [2–16]. The *seeding* scheme can be used in two distinct ways: tracking several seeds differing in size at a given  $(T, P)$  or studying a seed with a fixed size at different  $(T, P)$ . We found that the first protocol is more suitable when the critical size does not change significantly with the thermodynamic state point (i.e.  $\partial N_c / \partial P \sim 0$  or  $\partial N_c / \partial T \sim 0$ ) and we adopted it to identify  $N_c$  at most of the negative pressures. On the other hand, the second protocol (fixed seed simulated at different  $(T, P)$ ) works well when the critical size is sensitive to changes of  $T$  and/or  $P$ , as observed at positive pressures, and has been adopted in this regime.

To create the initial configuration for a single *seeding* run we first equilibrate separately bulk liquid water and bulk ice at the  $T$  and  $P$  of interest. Then, we create a spherical cavity of radius  $R$  within the bulk liquid water and insert in the empty space a spherical seed of a slightly smaller radius extracted from the bulk ice. The system is quickly equilibrated at constant volume for  $\sim 10$  ps keeping the ice-molecules motionless, which allows us to equilibrate the interface. Finally, we simulate the system in the  $NPT$  ensemble, where the pressures is applied isotropically.

In the following we show the estimation of  $N_c$  according to our *seeding* simulations.

| 230 K |              |       |            | 240 K |              |       |            | 250 K |              |       |            |
|-------|--------------|-------|------------|-------|--------------|-------|------------|-------|--------------|-------|------------|
| $N_c$ | $\Delta N_c$ | $P$   | $\Delta_P$ | $N_c$ | $\Delta N_c$ | $P$   | $\Delta_P$ | $N_c$ | $\Delta N_c$ | $P$   | $\Delta_P$ |
| 3284  | 0            | 1550  | 50         | 4360  | 0            | 1050  | 50         | 5160  | 70           | 450   | 50         |
| 2860  | 300          | 1500  | 0          | 3560  | 0            | 1000  | 100        | 4150  | 70           | 425   | 25         |
| 2590  | 0            | 1450  | 50         | 2750  | 700          | 900   | 0          | 3570  | 500          | 300   | 0          |
| 2105  | 400          | 1400  | 0          | 2003  | 0            | 700   | 100        | 3095  | 70           | 200   | 100        |
| 1610  | 0            | 1300  | 100        | 1690  | 0            | 650   | 50         | 1920  | 50           | -150  | 50         |
| 1022  | 450          | 900   | 0          | 1380  | 0            | 650   | 50         | 1760  | 50           | -300  | 100        |
| 485   | 0            | 550   | 50         | 1520  | 150          | 600   | 0          | 1600  | 150          | -400  | 0          |
| 186   | 25           | -100  | 0          | 1085  | 250          | 500   | 0          | 1370  | 50           | -450  | 150        |
| 210   | 25           | -300  | 0          | 797   | 0            | 250   | 50         | 1280  | 50           | -500  | 0          |
| 236   | 50           | -500  | 0          | 734   | 105          | 200   | 0          | 1275  | 150          | -600  | 0          |
| 225   | 35           | -700  | 0          | 662   | 70           | 100   | 0          | 1164  | 60           | -700  | 0          |
| 237   | 35           | -900  | 0          | 582   | 0            | 1     | 100        | 1093  | 30           | -800  | 0          |
| 165   | 55           | -1300 | 0          | 531   | 40           | -100  | 0          | 915   | 70           | -1000 | 0          |
| 150   | 25           | -1500 | 0          | 503   | 0            | -200  | 100        | 950   | 50           | -1300 | 0          |
| 189   | 80           | -1700 | 0          | 442   | 70           | -300  | 0          | 810   | 30           | -1400 | 100        |
| 235   | 50           | -2300 | 0          | 425   | 50           | -500  | 0          | 802   | 70           | -1500 | 0          |
| 277   | 50           | -2700 | 0          | 432   | 35           | -700  | 0          | 925   | 150          | -1700 | 0          |
| 307   | 35           | -3000 | 0          | 353   | 90           | -900  | 0          | 1035  | 75           | -1900 | 0          |
|       |              |       |            | 415   | 30           | -1100 | 0          | 1050  | 75           | -2500 | 0          |
|       |              |       |            | 393   | 20           | -1300 | 0          | 1200  | 75           | -2800 | 0          |
|       |              |       |            | 390   | 45           | -1500 | 0          |       |              |       |            |
|       |              |       |            | 310   | 45           | -1700 | 0          |       |              |       |            |
|       |              |       |            | 323   | 35           | -1900 | 0          |       |              |       |            |
|       |              |       |            | 462   | 55           | -2300 | 0          |       |              |       |            |
|       |              |       |            | 455   | 80           | -2500 | 0          |       |              |       |            |
|       |              |       |            | 516   | 35           | -2700 | 0          |       |              |       |            |
|       |              |       |            | 548   | 40           | -2900 | 0          |       |              |       |            |

TABLE I. Seeding results.  $\Delta N_c$  and  $\Delta_P$  are the uncertainty of the critical nucleus size and pressure respectively.

# MISLABELING CALCULATION

In Fig. 1 we report the % of mislabeled solid and liquid molecules, according to the threshold  $\bar{q}_{6,t}$  of the  $\bar{q}_6$  order parameter. The value of  $\bar{q}_{6,t}$  is determined from the crossing of the mislabeling curves of ice and liquid water in the bulk. For any  $P$  the optimal value of  $\bar{q}_{6,t}$  is well fitted by the expression  $\bar{q}_{6,t}(P) = a_{q_6}(T) - b_{q_6}(T) \exp(c_{q_6}(T)P)/[d_{q_6}(T) + \exp(c_{q_6}(T)P)]$  (see Fig. 2 of SM). The fitting parameters are reported in Tab. II.

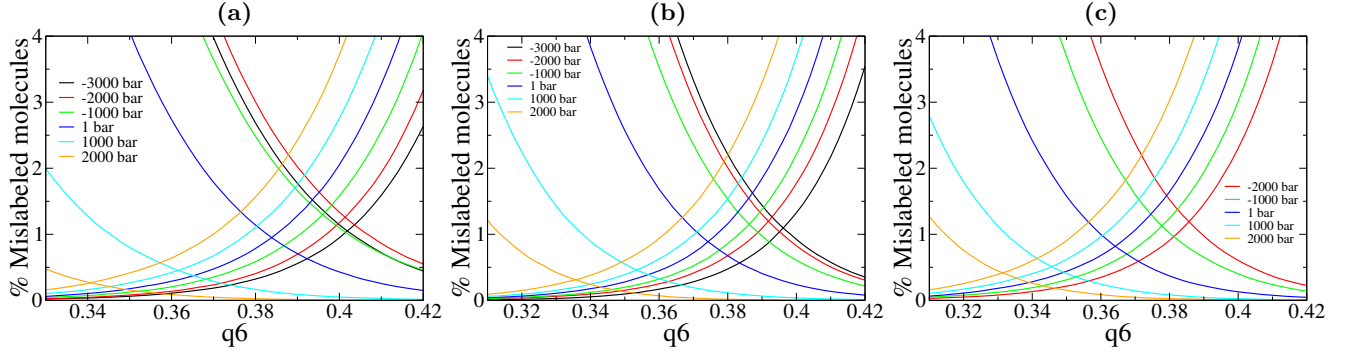

FIG. 1. Percentage of mislabeled molecules for each phase at  $T = 230$  K (a),  $T = 240$  K (b) and  $T = 250$  K (c). Data are over equilibrium simulations of 3820 molecules in the liquid phase, and 4032 molecules in the solid Ih phase.

| $T$ [K] | $a_{q_6}(T)$ | $b_{q_6}(T)$ | $c_{q_6}(T)$ | $d_{q_6}(T)$ |
|---------|--------------|--------------|--------------|--------------|
| 230     | 0.401839     | 0.0765991    | 0.00127229   | 3.29737      |
| 240     | 0.396191     | 0.0772493    | 0.00106575   | 2.35767      |
| 250     | 0.392375     | 0.0776309    | 0.000938774  | 1.7289       |

TABLE II. Fitting parameters for the  $\bar{q}_{6,t}$ .

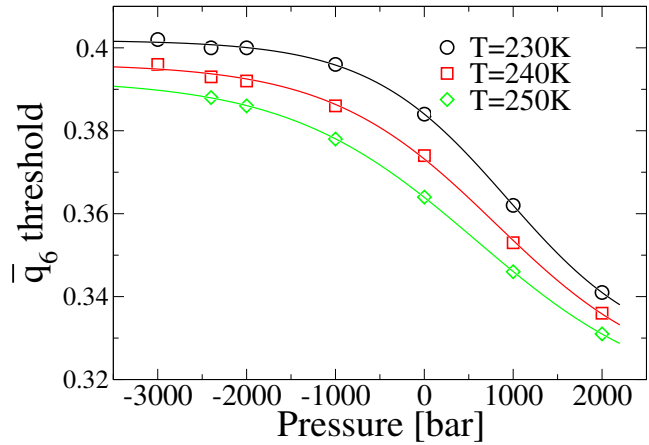

FIG. 2. Threshold  $\bar{q}_{6,t}$  for the  $\bar{q}_6$  order parameter as function of  $P$ , for different temperatures. Curves are fitted according to the expression reported in the SM.

# CALCULATION OF $\Delta\mu$

The difference between the chemical potentials of the liquid phase  $\mu_l$  and the solid phase  $\mu_s$  along an isotherm, at the desired pressure  $P$ , is given by

$$\Delta\mu(P) \equiv \mu_l(P) - \mu_s(P) = \int_{P_{\text{coex}}}^P [v_{\text{liq}}^{\text{mol}}(P') - v_{\text{ice}}^{\text{mol}}(P')] dP' \quad , \quad (1)$$

being  $P_{\text{coex}}$  the coexistence pressure at the temperature  $T$ ,  $v_{\text{liq}}^{\text{mol}}$  the molecular volume of the liquid phase,  $v_{\text{ice}}^{\text{mol}}$  the molecular volume of the solid phase. The  $P$  dependence of  $v_{\text{liq}}^{\text{mol}}$  and  $v_{\text{ice}}^{\text{mol}}$  are shown in Fig. 3a,b. Data are fitted with 9<sup>th</sup> order polynomials, whose coefficient are reported in Tab III. It is worth noting that, along the isotherms of the liquid phase shown in Fig. 3a, the volume data cross each other at positive pressures and negative pressures. This is due to the presence of a temperature of maximum density and a temperature of minimum density, both observed upon isobaric cooling. According to our data, we have that  $v_{\text{liq}}^{\text{mol}}(T = 240\text{K}) = v_{\text{liq}}^{\text{mol}}(T = 250\text{K})$  both at  $P \sim 1500$  bar and  $P \sim -2070$  bar, and  $v_{\text{liq}}^{\text{mol}}(T = 230\text{K}) = v_{\text{liq}}^{\text{mol}}(T = 240\text{K})$  both at  $P \sim 1650$  bar and  $P \sim -1890$  bar. The crossing at positive pressures indicates the presence of a maximum in density, along the point ( $T \sim 245\text{K}, P \sim 1500$  bar) and ( $T \sim 235\text{K}, P \sim 1650$  bar), while the crossing at negative pressure points out the presence of a minimum in density at ( $T \sim 245\text{K}, P \sim -2070$  bar) and ( $T \sim 235\text{K}, P \sim -1890$  bar). Moreover, as shown in Fig. 3c-e,  $v_{\text{liq}}^{\text{mol}}$  and  $v_{\text{ice}}^{\text{mol}}$  intersects at fixed  $T$ , marking the maximum of  $\Delta\mu$  shown in Fig. 5a of the main text. We found that  $v_{\text{liq}}^{\text{mol}} = v_{\text{ice}}^{\text{mol}}$  at ( $T = 230\text{K}, P \sim -1110$  bar), ( $T = 240\text{K}, P \sim -1420$  bar) and ( $T = 250\text{K}, P \sim -1605$  bar).

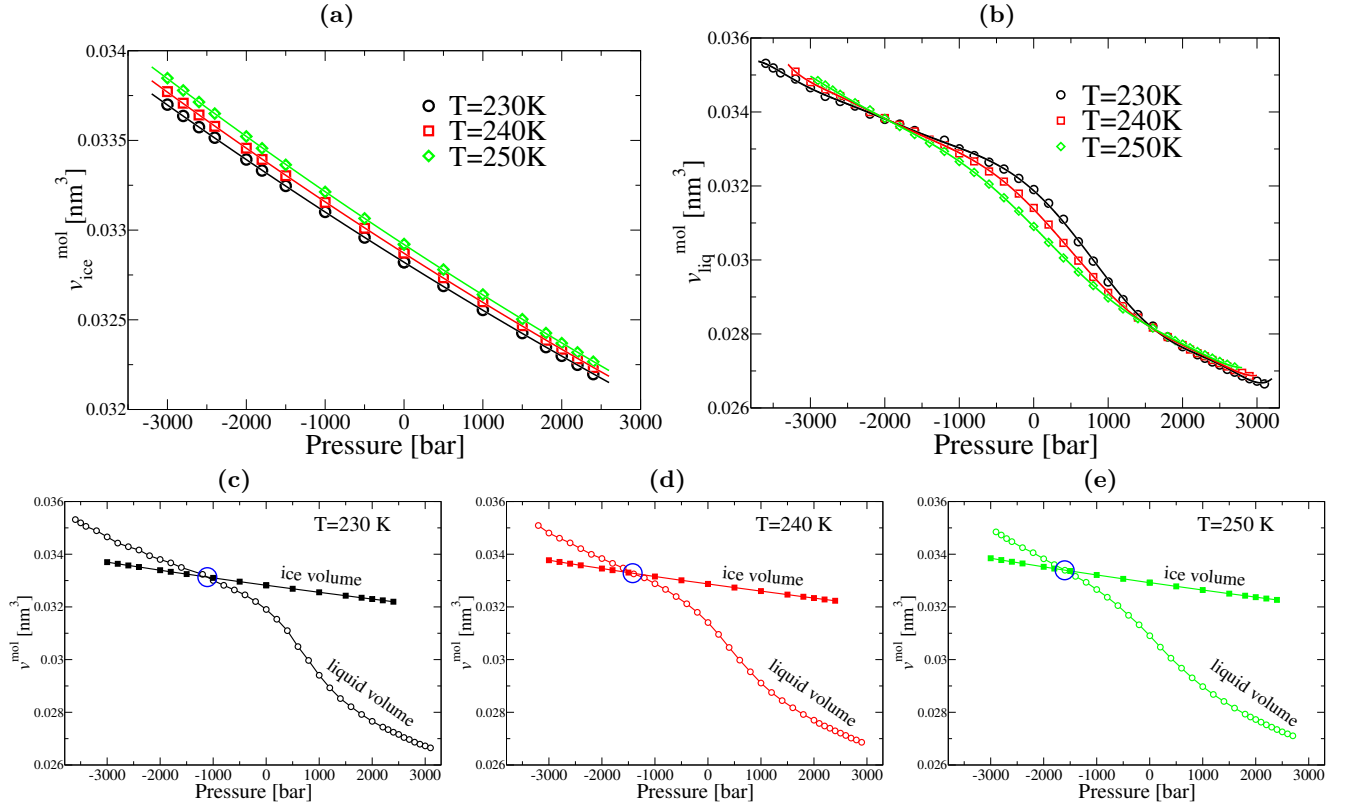

FIG. 3. Molecular volume of ice Ih  $v_{\text{ice}}^{\text{mol}}$  (a) and liquid water  $v_{\text{liq}}^{\text{mol}}$  (b) as function of pressure, for different temperatures. Data are calculated with  $NPT$  runs spanning up to 200 ns of a bulk liquid phase of 3840 molecules, and a bulk of 4032 ice molecules. Lines are polynomial fits described in the text and in TAB. III. Panels (c-e) show the molecular volume  $v^{\text{mol}}$  of liquid (open circles) and solid phase (full squares) at  $T = 230\text{K}$  (c),  $T = 240\text{K}$  (d) and  $T = 250\text{K}$  (e). Blue circles mark the crossing between  $v_{\text{ice}}^{\text{mol}}$  and  $v_{\text{liq}}^{\text{mol}}$ .

| $v$                           | $T$ | $a_v(T)$              | $b_v(T)$              | $c_v(T)$              | $d_v(T)$              | $e_v(T)$              | $f_v(T)$              | $g_v(T)$              | $h_v(T)$              | $i_v(T)$             | $l_v(T)$             |
|-------------------------------|-----|-----------------------|-----------------------|-----------------------|-----------------------|-----------------------|-----------------------|-----------------------|-----------------------|----------------------|----------------------|
| [nm <sup>3</sup> ]            | [K] | ( $\times 10^{-34}$ ) | ( $\times 10^{-31}$ ) | ( $\times 10^{-27}$ ) | ( $\times 10^{-24}$ ) | ( $\times 10^{-20}$ ) | ( $\times 10^{-17}$ ) | ( $\times 10^{-13}$ ) | ( $\times 10^{-10}$ ) | ( $\times 10^{-6}$ ) | ( $\times 10^{-2}$ ) |
| $v_{\text{ice}}^{\text{mol}}$ | 250 | 0                     | 0                     | 0                     | 0                     | 0                     | 0                     | 0                     | 0.0676672             | -0.287745            | 3.29197              |
| $v_{\text{ice}}^{\text{mol}}$ | 240 | 0                     | 0                     | 0                     | 0                     | 0                     | 0                     | 0                     | 0.0634812             | -0.280247            | 3.28709              |
| $v_{\text{ice}}^{\text{mol}}$ | 230 | 0                     | 0                     | 0                     | 0                     | 0                     | 0                     | 0                     | 0.0607871             | -0.273831            | 3.28217              |
| $v_{\text{liq}}^{\text{mol}}$ | 250 | 0                     | 3.53928               | 1.56695               | -5.80737              | -2.9843               | 3.84266               | 2.24401               | -1.1388               | -2.04296             | 3.08979              |
| $v_{\text{liq}}^{\text{mol}}$ | 240 | 0                     | 7.91325               | 1.33479               | -17.2535              | -2.80532              | 13.7737               | 2.29159               | -4.77538              | -2.08529             | 3.13703              |
| $v_{\text{liq}}^{\text{mol}}$ | 230 | 2.46393               | 10.0899               | -5.35123              | -24.2833              | 3.44422               | 21.2156               | -0.0287716            | -8.12152              | -1.80442             | 3.18724              |

TABLE III. Coefficient of the polynomial fit for the molecular volume  $v^{\text{mol}}$  of liquid and solid phases, shown in Fig. 3. The fitting polynomial as function of  $P$  is  $a_v(T)P^9 + b_v(T)P^8 + c_v(T)P^7 + d_v(T)P^6 + e_v(T)P^5 + f_v(T)P^4 + g_v(T)P^3 + h_v(T)P^2 + i_v(T)P + l_v(T)$ .

### FIT OF $N_c$

The pressure dependence of the ice critical size  $N_c$  has been fitted according to the expression  $N_c(T, P) = a_{N_c}(T)P^2 + b_{N_c}(T)P + c_{N_c}(T) + d_{N_c}(T)\exp[e_{N_c}(T)(P + h_{N_c}(T))]$ . The fitting parameters are shown in Tab. IV

| $T$ | $a_{N_c}(T)$         | $b_{N_c}(T)$ | $c_{N_c}(T)$      | $d_{N_c}(T)$ | $e_{N_c}(T)$         | $h_{N_c}(T)$      |
|-----|----------------------|--------------|-------------------|--------------|----------------------|-------------------|
| [K] | ( $\times 10^{-4}$ ) |              | ( $\times 10^2$ ) |              | ( $\times 10^{-3}$ ) | ( $\times 10^3$ ) |
| 230 | 0.341809             | 0.0797471    | 2.35066           | 0.85         | 2.46                 | 1.72              |
| 240 | 1.32674              | 0.368069     | 5.7071            | 9.5          | 4.6                  | 0.22              |
| 250 | 3.3502               | 1.147        | 18.3463           | 0.3          | 4.5                  | 1.57              |

TABLE IV. Fitting parameters of the curves  $N_c(T, P)$ .

### FIT OF $D$

The pressure dependence of the diffusion coefficient  $D(T, P)$  is given by  $D(T, P) = a_D(T) + \exp[b_D(T)P]/\{c_D(T) + d_D(T)\exp[b_D(T)P]\} + [e_D(T)P + f_D(T)P^2]/\{1 + \exp[h_D(T)P]\}$ , with parameters shown in Tab. V

| $T$ | $a_D(T)$             | $b_D(T)$             | $c_D(T)$  | $d_D(T)$  | $e_D(T)$             | $f_D(T)$              | $h_D(T)$             |
|-----|----------------------|----------------------|-----------|-----------|----------------------|-----------------------|----------------------|
| [K] | ( $\times 10^{-4}$ ) | ( $\times 10^{-3}$ ) |           |           | ( $\times 10^{-7}$ ) | ( $\times 10^{-12}$ ) | ( $\times 10^{-3}$ ) |
| 230 | 8.99447              | 3.00448              | 193.8014  | 13.68375  | 1.7342152            | 0                     | 125.5709             |
| 240 | 34.87718             | 2.630391             | 28.8107   | 8.2971    | 5.737374             | 7.8152591             | 34.16511             |
| 250 | 311.085              | 2.4591358            | 8.3357863 | 7.5807725 | 145.64959            | 2217.4348             | 2.824802             |

TABLE V. Fitting parameters of the curves  $D(T, P)$ .

# ATTACHMENT RATE $f^+$

The attachment rate  $f^+$  can be rigoursly computed from the expression proposed by Auer and Frenkel[17]

$$f_{AF}^+ = \frac{\langle (N(t) - N(0))^2 \rangle}{2t} \quad (2)$$

and approximated by the equation

$$f^+ = \frac{24DN_c^{2/3}}{\lambda^2} \quad (3)$$

where  $D$  is the diffusion coefficient of the supercooled liquid,  $N_c$  the size of the critical nucleus, and  $\lambda \equiv 3.8\text{\AA}$  is a characteristic length of the order of a molecular diameter [4]. In a previous work, we have applied this approximation in nucleation of ice at positive pressures finding good agreement with the rigorous procedure [4]. Here, we test it at negative pressures, also finding good agreement as can be seen in Table VI. In particular, along the 240 K isotherm, we calculate  $f^+$  for three different negative pressures: -300 bar, -1700 bar, and -2900 bar.

| $P$ (bar) | $f_{AF}^+$ (ns <sup>-1</sup> ) | $f^+$ (ns <sup>-1</sup> ) |
|-----------|--------------------------------|---------------------------|
| -300      | 129.5                          | 111.4                     |
| -1700     | 22.1                           | 16.6                      |
| -2900     | 15.0                           | 13.9                      |

TABLE VI. Attachment rate computed according the rigorous Eq. 2 and approximated by the Eq. 3.

# ERROR BARS FOR $\Delta G$ AND $\log_{10}J$

In Fig. 4, we have a closer look at the minima of  $\Delta G$  and maxima of  $\log_{10}J$ . We also include error bars. As can be seen, the uncertainty is not enough to cover the non-monotonic behavior.

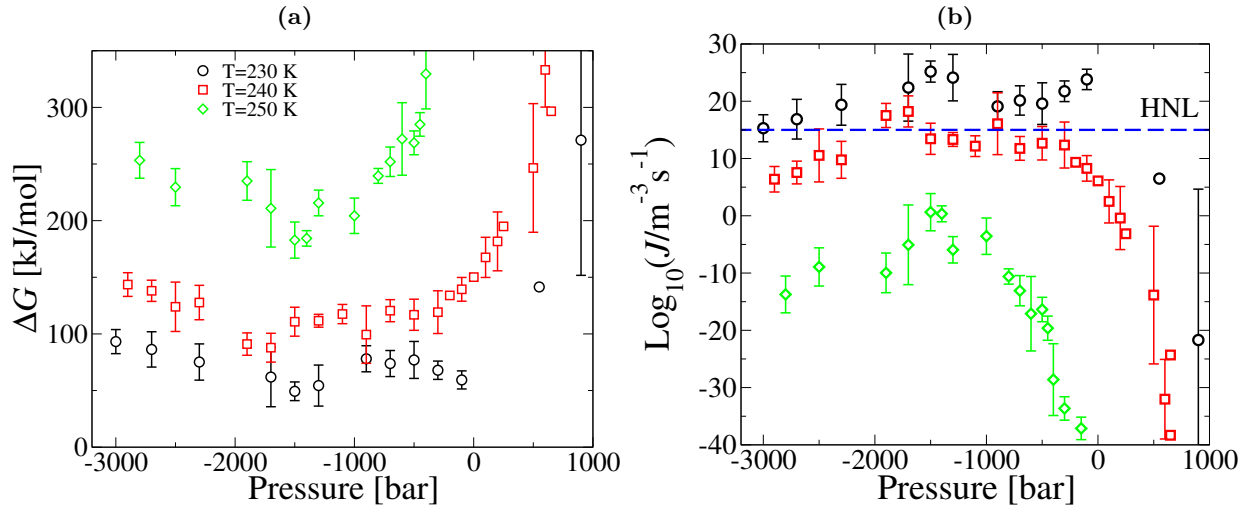

FIG. 4. Zoom in Fig. 3d) and 4b) from main text. Here, a) free energy barrier  $\Delta G$  and b) the logarithm of the nucleation rate  $J$ . Error bars are included. The same legend applies in both panels.

- 
- [1] X.-M. Bai and M. Li, The Journal of Chemical Physics **122**, 224510 (2005).
  - [2] E. Sanz, C. Vega, J. R. Espinosa, R. Caballero-Bernal, J. L. F. Abascal, and C. Valeriani, Journal of the American Chemical Society **135**, 15008 (2013).
  - [3] J. R. Espinosa, C. Vega, and E. Sanz, The Journal of Physical Chemistry C **122**, 22892 (2018).
  - [4] J. R. Espinosa, E. Sanz, C. Valeriani, and C. Vega, The Journal of chemical physics **141**, 18C529 (2014).
  - [5] J. R. Espinosa, C. Vega, C. Valeriani, and E. Sanz, The Journal of Chemical Physics **144**, 034501 (2016).
  - [6] J. R. Espinosa, C. Navarro, E. Sanz, C. Valeriani, and C. Vega, The Journal of Chemical Physics **145**, 211922 (2016).
  - [7] N. E. Zimmermann, B. Vorselaars, D. Quigley, and B. Peters, Journal of the American Chemical Society **137**, 13352 (2015).
  - [8] B. C. Knott, V. Molinero, M. F. Doherty, and B. Peters, Journal of the American Chemical Society **134**, 19544 (2012).
  - [9] Y. Lifanov, B. Vorselaars, and D. Quigley, The Journal of Chemical Physics **145**, 211912 (2016).
  - [10] F. Leoni, R. Shi, H. Tanaka, and J. Russo, The Journal of Chemical Physics **151**, 044505 (2019).
  - [11] R. G. Pereyra, I. Szleifer, and M. A. Carignano, The Journal of chemical physics **135**, 034508 (2011).
  - [12] P. Montero de Hijos, J. R. Espinosa, E. Sanz, and C. Vega, The Journal of Chemical Physics **151**, 144501 (2019).
  - [13] P. Montero de Hijos, J. R. Espinosa, V. Bianco, E. Sanz, and C. Vega, The Journal of Physical Chemistry C **124**, 8795 (2020).
  - [14] A. O. Tipeev, E. D. Zanotto, and J. P. Rino, The Journal of Physical Chemistry C **122**, 28884 (2018).
  - [15] T. Dasgupta, G. M. Coli, and M. Dijkstra, ACS Nano **14**, 3957 (2020).
  - [16] H. Niu, L. Bonati, P. M. Piaggi, and M. Parrinello, Nature Communications **11**, 2654 (2020).
  - [17] S. Auer and D. Frenkel, Nature **409**, 1020 (2001).
